# Supplementary material for: Characterizing Superradiant Phase of the Quantum Rabi Model
Source: arXiv:2207.13285 source file (2022-07-27)
Supplement: Supplementary file 1 [file SM.pdf]

# Supplementary Material for "Characterizing Superradiant Phase of the Quantum Rabi Model"

Yun-Tong Yang[1,2] and Hong-Gang Luo[1,2,3]

[1] School of Physical Science and Technology, Lanzhou University, Lanzhou 730000, China
[2] Lanzhou Center for Theoretical Physics and Key Laboratory of Theoretical Physics of Gansu Province, Lanzhou University, Lanzhou 730000, China
[3] Beijing Computational Science Research Center, Beijing 100084, China

### A. The convergence of our method

In the main text, we provide a scheme consisting of two successive diagonalization to accurately obtain energy levels and wavefunctions of the QRM, where the first is made exactly in the two-level space and the second is done in the truncated Fock space. Therefore, the convergence of our approach depends on the size of the truncated Fock basis, i. e. the size of the $N \times N$ matrix of Eq. (10) in the paper. In order to assess the convergence and accuracy of our scheme, we compare the energy spectrum obtained from numerical ED with our calculated results by using the formula as follows

$$\delta E = E_{ED} - E_{ours} \tag{1}$$

The criterion of whether the system converges is whether $\delta E$ equals to zero. Figure 1 shows the $\delta E$ of the ground state and the other nine low-lying excited states as functions of the coupling strengths scaled by $g_c = \sqrt{1+\sqrt{1+\frac{\Delta^2}{16}}}$. We choose four different types of the truncated Fock basis: 10, 20, 30 and 50. For the ground-state and the first four excited states, the results show that the system converges well in full parameter regime when the truncated basis is taken 30, as shown in Fig. 1(a-e). For higher excited states, from the fifth excited state to the ninth excited state, a larger truncated matrix is needed to enable the system to converge and the results show when the truncated basis is taken 50 our method could converge well, as shown in Fig. 1(f-j). In our present paper, the truncated basis is taken 50, so our calculated results are accurate and reliable.

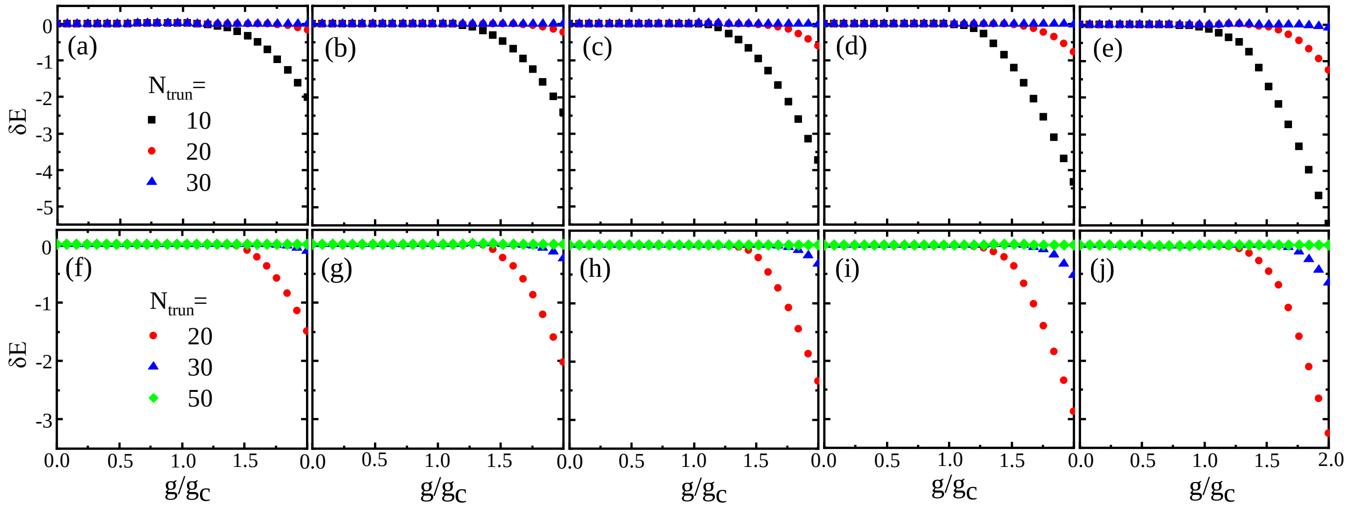


FIG. 1. The difference of energy levels between ED and our scheme of the ground state and the other nine low-lying excited states as functions of the coupling strengths scaled by $g_c = \sqrt{1+\sqrt{1+\frac{\Delta^2}{16}}}$. We choose four different sizes of the truncated Fock basis: 10, 20, 30 (the first row, a-e) and 20, 30, 50 (the second row, f-j).

### B. Fitting parameters of the photon population

With accurate wavefunctions at hand, we calculate the photon population and the results show some characteristic behaviors, as shown in Fig. 3 and Fig. 4 in the main text. In order to check how the photons populate, we borrow three typical level statistical distributions in random matrix theory. The standard formulas are as follows

$$P_P(s) = e^{-s}, \tag{2}$$
$$P_{GUE}(s) = \frac{32}{\pi^2} s^2 e^{-\frac{4s^2}{\pi}}, \tag{3}$$
$$P_{GOE}(s) = \frac{\pi}{2} s e^{-\frac{\pi s^2}{4}}, \tag{4}$$

which correspond to the Poissonian statistics, the statistics of GUE and GOE. The variable $s$ denotes the energy intervals of adjacent levels in the original definition. We replace it, however, by the Fock basis $n$. We make an overall enlargement of the formulas by multiplying the parameter $b$, and replace $n$ with $a(n+c)$ for the GUE and GOE distributions. The specific formulas we used are as follows

$$P_P(n) = be^{-an}, \tag{5}$$
$$P_{GUE}(n) = b\frac{32}{\pi^2}(a(n+c))^2 e^{-\frac{4(a(n+c))^2}{\pi}}, \tag{6}$$
$$P_{GOE}(n) = b\frac{\pi}{2}(a(n+c)) e^{-\frac{\pi(a(n+c))^2}{4}}. \tag{7}$$

The values of specific fitting parameters are listed in Table 1.

| Fock basis | Even | Odd | Even | Odd | Even | Odd | Even | Odd |
|---|---|---|---|---|---|---|---|---|
| FIG. 3 | (a2) | | (b2) | | (c2) | | (d2) | |
| a | 0.358 | 0.372 | 0.550 | 0.369 | 0.565 | 0.345 | 0.586 | 0.321 |
| b | 0.441 | 0.168 | 0.585 | 0.088 | 0.651 | 0.042 | 0.670 | 0.027 |
| FIG. 3 | (a3) | | (b3) | | (c3) | | (d3) | |
| a | 0.166 | 0.166 | 0.140 | 0.140 | 0.119 | 0.119 | 0.101 | 0.101 |
| b | 0.209 | 0.137 | 0.188 | 0.104 | 0.162 | 0.074 | 0.139 | 0.060 |
| c | 0.458 | 0.218 | 0 | -0.746 | -3.429 | -3.827 | -6.426 | -6.900 |
| FIG. 4 | (a) | | (b) | | (c) | | (d) | |
| a | 0.140 | 0.140 | 0.140 | 0.140 | 0.200 | 0.200 | 0.200 | 0.200 |
| b | 0.188 | 0.104 | 0.100 | 0.195 | 0.150 | 0.087 | 0.090 | 0.146 |
| c | 0 | -0.746 | -0.600 | -0.396 | -7.668 | -7.822 | -7.759 | -7.686 |

TABLE I. The fitting parameters of the Poissonian-like statistics, the statistics of GUE-like and GOE-like in Fig. 3 and Fig. 4 of the main text.
